# Supplementary material for: Train Till You Drop: Towards Stable and Robust Source-free Unsupervised 3D Domain Adaptation
Source: arXiv:2409.04409 source file (2024-09-06)
Supplement: Supplementary file 1 [file AppendixCameraReady.tex]

\documentclass[runningheads]{llncs}
% Include basic ECCV package
 
% TODO REVIEW: Insert your submission number below by replacing '*****'
% TODO FINAL: Comment out the following line for the camera-ready version
%\usepackage[review,year=2024,ID=2968]{eccv}
% TODO FINAL: Un-comment the following line for the camera-ready version
\usepackage{eccv}

% OPTIONAL: Un-comment the following line for a version which is easier to read
% on small portrait-orientation screens (e.g., mobile phones, or beside other windows)
%\usepackage[mobile]{eccv}

% ---------------------------------------------------------------
% Other packages

% Commonly used abbreviations (\eg, \ie, \etc, \cf, \etal, etc.)
\usepackage{eccvabbrv}

% Include other packages here, before hyperref.
\usepackage{graphicx}
\usepackage{booktabs}

% The "axessiblity" package can be found at: https://ctan.org/pkg/axessibility?lang=en
\usepackage[accsupp]{axessibility}  % Improves PDF readability for those with disabilities.

% ---------------------------------------------------------------
% Hyperref package

% It is strongly recommended to use hyperref, especially for the review version.
% Please disable hyperref *only* if you encounter grave issues.
% hyperref with option pagebackref eases the reviewers' job, but should be disabled for the final version.
%
% If you comment hyperref and then uncomment it, you should delete
% main.aux before re-running LaTeX.
% (Or just hit 'q' on the first LaTeX run, let it finish, and you
%  should be clear).

% TODO FINAL: Comment out the following line for the camera-ready version
%\usepackage[pagebackref,breaklinks,colorlinks,citecolor=eccvblue]{hyperref}
% TODO FINAL: Un-comment the following line for the camera-ready version
\usepackage{hyperref}

% Support for ORCID icon
\usepackage{orcidlink}
\input{commands}

\title{\titletext\\
\textit{--- Supplementary Material ---}}

% TODO REVIEW: If the paper title is too long for the running head, you can set
% an abbreviated paper title here. If not, comment out.
%\titlerunning{TTYD: Train Till You Drop}
\titlerunning{TTYD: Towards Stable and Robust
3D SFUDA}

% TODO FINAL: Replace with your author list. 
% Include the authors' OCRID for the camera-ready version, if at all possible.
\author{Bj\"orn Michele\inst{1,2}\orcidlink{0009-0004-1902-6232} \and
Alexandre Boulch\inst{1}\orcidlink{0000-0002-4196-9665} \and
Tuan-Hung Vu\inst{1}\orcidlink{0000-0002-9765-8233} 
\and 
Gilles Puy \inst{1}%\orcidlink{xxxx-xxxx-xxxx-xxxx}
\and 
Renaud~Marlet \inst{1,3}\orcidlink{0000-0003-1612-1758} \and
Nicolas Courty \inst{2}\orcidlink{0000-0003-1353-0126}}

% TODO FINAL: Replace with an abbreviated list of authors.
\authorrunning{B.~Michele et al.}
% First names are abbreviated in the running head.
% If there are more than two authors, 'et al.' is used.

% TODO FINAL: Replace with your institution list.
\institute{Valeo.ai, Paris, France  
\and
CNRS, IRISA, Univ.\ Bretagne Sud, Vannes, France
\and
LIGM, Ecole des Ponts, Univ Gustave Eiffel, CNRS, Marne-la-Vall\'ee, France}

\begin{document}
\maketitle

%%%%%%%%% MAIN PAPER
% WARNING: do not forget to delete the supplementary pages from your submission 
\input{sections/appendix}
\FloatBarrier
{\small
\bibliographystyle{splncs04}
\bibliography{egbib}
}

\end{document}
