# Supplementary material for: Train Till You Drop: Towards Stable and Robust Source-free Unsupervised 3D Domain Adaptation
Source: arXiv:2409.04409 source file (2024-09-06)
Supplement: Supplementary file 2 [file AppendixForReview.tex]

\documentclass[runningheads]{llncs}
% Include basic ECCV package
 
% TODO REVIEW: Insert your submission number below by replacing '*****'
% TODO FINAL: Comment out the following line for the camera-ready version
\usepackage[review,year=2024,ID=2968]{eccv}
% TODO FINAL: Un-comment the following line for the camera-ready version
%\usepackage{eccv}

% OPTIONAL: Un-comment the following line for a version which is easier to read
% on small portrait-orientation screens (e.g., mobile phones, or beside other windows)
%\usepackage[mobile]{eccv}

% ---------------------------------------------------------------
% Other packages

% Commonly used abbreviations (\eg, \ie, \etc, \cf, \etal, etc.)
\usepackage{eccvabbrv}

% Include other packages here, before hyperref.
\usepackage{graphicx}
\usepackage{booktabs}

% The "axessiblity" package can be found at: https://ctan.org/pkg/axessibility?lang=en
\usepackage[accsupp]{axessibility}  % Improves PDF readability for those with disabilities.

% ---------------------------------------------------------------
% Hyperref package

% It is strongly recommended to use hyperref, especially for the review version.
% Please disable hyperref *only* if you encounter grave issues.
% hyperref with option pagebackref eases the reviewers' job, but should be disabled for the final version.
%
% If you comment hyperref and then uncomment it, you should delete
% main.aux before re-running LaTeX.
% (Or just hit 'q' on the first LaTeX run, let it finish, and you
%  should be clear).

% TODO FINAL: Comment out the following line for the camera-ready version
\usepackage[pagebackref,breaklinks,colorlinks,citecolor=eccvblue]{hyperref}
% TODO FINAL: Un-comment the following line for the camera-ready version
%\usepackage{hyperref}

% Support for ORCID icon
\usepackage{orcidlink}
\input{commands}

\title{\titletext\\
\textit{--- Supplementary Material ---}}

\begin{document}
\maketitle

%\input{sections/abstract}

%%%%%%%%% MAIN PAPER
%\input{main}

% WARNING: do not forget to delete the supplementary pages from your submission 
\input{sections/appendix}
\FloatBarrier
{\small
\bibliographystyle{splncs04}
\bibliography{egbib}
}

\end{document}
