# Supplementary material for: Train Till You Drop: Towards Stable and Robust Source-free Unsupervised 3D Domain Adaptation
Source: arXiv:2409.04409 source file (2024-09-06)
Supplement: Supplementary file 3 [file prepare_supp_appendix.tex]

\bgroup
\hypersetup{linkbordercolor=black}
\hypersetup{hidelinks}
\tableofcontents
\egroup
